# Supplementary material for: A reddening-free method to estimate the $^{56}$Ni mass of Type Ia supernovae
Source: arXiv:1601.04874 source file (2016-01-19)
Supplement: Supplementary file 1 [file appendix.tex]

\section{Principal Component Analysis in the combined fit}

In section \ref{sssec-cf} we tried to simultaneously fit the $t_2$ in $Y$ and $J$ to obtain combined constraints on $L_{max}$, using a multivariate fit to both the $J$ and $Y$ band data. However, the multivariate regression returns estimates with insignificant $t$-statistics and a high standard error. Moreover, the slope estimated for the $Y$ band $t_2$, in the multivariate fit, is \emph{negative} which is incorrect since the $t_2(Y)$ has a positive correlation with $L_{max}$. 

These estimates for the multivariate regression are incorrect due to the problem of multicollinearity. This arises due to the strong correlation between the predictor variables, in this case, $t_2$ $Y$ and $J$. In order to circumvent this problem, we apply a principal component analysis (PCA) to the two variables and transform them, along the axis of maximum variance,  into uncorrelated principal components (PCs). 

We use  a Python package \emph{sci-kit learn} to decompose the variables into a PC. We derive a linear relation between the PC and the $L_{max}$ values in Table \ref{tab:mni}. 
The measured $t_2$ for heavily reddened objects are transformed in the direction of the PC and the error from the slope of the linear relation is propagated. For the final estimated $L_{max}$, we add the mean $L_{max}$ for the objects in the low-reddening sample. The error on the mean is calculated by bootstrap resampling.  
We find that the PCA estimates give a marginal improvement on the error for the final $M_{{^56}Ni}$ value. 

Table \ref{tab:pca_red} presents the constraints from the PCA estimates. We can see that error bars are smaller than in Table \ref{tab:red}

\begin{table}
\begin{minipage}{70mm}
\begin{center}
\caption{$M_{^{56}Ni}$ estimates for 5 objects with high values of $E(B-V)_{host}$ using PCA (see text). The constraints have smaller errors than the estimates in Table \ref{tab:red}}

\begin{tabular}{llcccrr}
\hline
SN & $M_{^{56}Ni}$ (inferred) & $\sigma$  \\
\hline
SN1986G	& 0.34 & 0.08	\\
SN2005A	& 0.56	&  0.10  \\
SN2006X	& 0.57 & 0.10  \\\
SN2008fp &  0.63 & 0.11 \\
SN2014J	& 0.66	& 0.12 \\

\hline
\end{tabular}
\label{tab:pca_red}
\end{center}
\end{minipage}
\end{table}

%----------------------------------------------------------------------%

\section{Markov Chain Monte Carlo fits to linear model}

In this section we outline the procedure to fit a linear model to the observed $L_{max}$-$t_2$ relation for the low-reddening sample. We use a bayesian framework for parameter estimation for the slope and intercept. We sample the posterior probability distribution using two different numerical methods. Firstly, we use an affine invariant Markov Chain Monte Carlo (MCMC) package called \emph{emcee} \citep{FM13}. The theoretical background for affine invariant MCMC sampling is presented in \citet{Goodman2010}. 

As a consistency check we also use a Bayesian method prescribed in \citet{Kelly2007}. 
The author uses a Gibbs Sampling method to generate random draws from the posterior probability distribution. The implementation allows propagating errors on both the $x$ and $y$ axes. It also accounts for heteroscedastic error measurements.
We find that using both results yields consistent estimates for the  $M_{{^56}Ni}$

\begin{table}
\begin{minipage}{70mm}
\begin{center}
\caption{$M_{^{56}Ni}$ measurements from MCMC sampling. We see an improvement in the error estimates compared to the values in Table \ref{tab:red}}
\begin{tabular}{llcccrr}
\hline
SN & $M_{^{56}Ni}$ (inferred) & $\sigma_{upper}$ & $\sigma_{lower}$  \\
\hline
SN1986G	& 0.32 & 0.07 & 0.05	\\
SN2005A	& 0.55	&  0.09 & 0.07  \\
SN2006X	& 0.57 & 0.10 & 0.08  \\\
SN2008fp &  0.63 & 0.11 & 0.08 \\
SN2014J	& 0.65	& 0.11 & 0.09 \\

\hline
\end{tabular}
\label{tab:mcmc}
\end{center}
\end{minipage}
\end{table}

Sampling the posterior distribution gives us the values for the slope and intercepts and we calculate the values of the $L_{max}$ from the samples and the measured $t_2$. We then use Arnett's rule with fixed rise to get a distribution of $M_{^{56}Ni}$ values. We take the highest posterior density (HPD) of the final $M_{^{56}Ni}$ as our best estimate and the errors are given by the region of 68 $\%$ confidence from the HPD.
